# Supplementary material for: BUDHIES I: characterizing the environments in and around two clusters at z~0.2
Source: arXiv:1302.1876 ancillary file (2013-03-24)
Supplement: Supplementary file 1 [file Spec_table_A2192_and_A963.pdf]

# 1 Online Table: measured redshifts and [OII] equivalent widths in Jaffé et al. (2012)

The table below contains the optical information for all the galaxies observed with the WHT for which a redshift was obtained. The columns are: Field (Abell 963 or 2192), Object ID,  $R$ -band magnitude,  $B$ -band magnitude, redshift, redshift quality, spectral type, and equivalent width of the [OII] emission line. The ID is preceded by “IJ” and contains the right ascension and declination of the INT photometry in hhmmss.ss and ddmmss.s format. All redshifts have an uncertainty of 0.0003. The redshift quality ranges from 1 to -2, only redshifts quality  $\geq -1$  are to be trusted. The type of spectra is also indicated: “em” stands for emission-line spectra, “ab” for absorption, “em+ab” means that there are both types of features clearly visible, “em/ab” when there is significantly more emission than absorption, “ab/em” in the opposite case, and “nan” when the galaxy spectra did not have clear features. The string “-” is placed when there are no EW[OII] measurements available (in the ASCII version of the table, the number “-11.11” is used instead).

| Field | ID                   | $R$<br>mag | $B$<br>mag | redshift | redshift<br>quality | type of<br>spectra | EW[OII] |
|-------|----------------------|------------|------------|----------|---------------------|--------------------|---------|
| A963  | IJ101507.08+385757.0 | 18.71      | 20.70      | 0.1478   | 1                   | ab                 | -       |
| A963  | IJ101507.13+390027.8 | 19.15      | 21.42      | 0.3632   | -1                  | em+ab              | 38.21   |
| A963  | IJ101509.18+390312.4 | 19.14      | 20.61      | 0.2987   | 1                   | em/ab              | 18.15   |
| A963  | IJ101509.74+390341.5 | 18.23      | 20.04      | 0.2984   | -1                  | ab/em              | 5.85    |
| A963  | IJ101510.60+385618.0 | 18.81      | 20.39      | 0.3011   | 1                   | em                 | 22.08   |
| A963  | IJ101513.23+390818.6 | 18.46      | 20.14      | 0.0946   | -1                  | ab                 | -       |
| A963  | IJ101515.62+390248.9 | 18.15      | 19.97      | 0.1205   | -2                  | nan                | -       |
| A963  | IJ101517.07+390601.9 | 18.66      | 19.74      | 0.2689   | -1                  | em/ab              | 16.42   |
| A963  | IJ101517.38+385336.8 | 18.11      | 19.91      | 0.1209   | 1                   | ab                 | -       |
| A963  | IJ101522.92+391146.3 | 18.82      | 20.43      | 0.3422   | -2                  | nan                | -       |
| A963  | IJ101523.40+390728.5 | 18.44      | 19.48      | 0.0488   | 1                   | em/ab              | 54.9    |
| A963  | IJ101523.79+385834.8 | 17.94      | 20.00      | 0.1469   | 1                   | ab                 | -       |
| A963  | IJ101524.93+384823.6 | 18.58      | 20.24      | 0.2154   | -1                  | ab/em              | 12.21   |
| A963  | IJ101527.38+385132.3 | 17.84      | 19.05      | 0.1218   | 1                   | ab                 | -       |
| A963  | IJ101527.90+390603.6 | 18.69      | 20.07      | 0.2054   | 1                   | em+ab              | 14.28   |
| A963  | IJ101528.63+385800.6 | 17.63      | 19.44      | 0.2344   | 1                   | ab                 | -       |
| A963  | IJ101530.63+391209.5 | 18.28      | 19.45      | 0.064    | -2                  | nan                | -       |
| A963  | IJ101530.85+385255.2 | 18.45      | 20.78      | 0.2013   | -2                  | nan                | -       |
| A963  | IJ101532.79+384805.1 | 18.47      | 20.75      | 0.206    | 1                   | ab                 | -       |
| A963  | IJ101533.95+384745.1 | 19.44      | 21.05      | 0.3202   | -1                  | em/ab              | 15.32   |
| A963  | IJ101534.02+391212.1 | 19.44      | 21.13      | 0.1257   | -2                  | nan                | -       |
| A963  | IJ101534.81+390912.0 | 18.22      | 20.46      | 0.1749   | 1                   | ab                 | -       |
| A963  | IJ101535.51+385436.7 | 18.82      | 20.20      | 0.2662   | 1                   | em/ab              | 32.58   |
| A963  | IJ101537.64+391353.0 | 19.43      | 20.83      | 0.2646   | 1                   | em/ab              | 11.77   |
| A963  | IJ101538.37+390115.1 | 18.59      | 20.02      | 0.0644   | 1                   | em                 | 55.05   |
| A963  | IJ101538.64+390150.4 | 17.25      | 18.64      | 0.993    | -2                  | nan                | -       |
| A963  | IJ101539.78+391608.8 | 18.38      | 20.76      | 0.2461   | 1                   | ab                 | -       |
| A963  | IJ101540.59+391633.6 | 19.45      | 20.90      | 0.2213   | 1                   | em+ab              | 12.5    |
| A963  | IJ101540.97+384851.6 | 19.13      | 20.87      | 0.2906   | -2                  | nan                | -       |
| A963  | IJ101541.30+391525.7 | 18.23      | 20.02      | 0.1762   | 1                   | em+ab              | 19.37   |
| A963  | IJ101541.85+391642.2 | 19.00      | 21.27      | 0.162    | -2                  | nan                | -       |
| A963  | IJ101544.32+384910.9 | 19.01      | 20.82      | 0.2064   | 1                   | em/ab              | 11.1    |
| A963  | IJ101546.37+390917.5 | 17.93      | 20.11      | 0.2039   | 1                   | ab                 | -       |
| A963  | IJ101547.85+391655.1 | 19.26      | 21.35      | 0.2447   | 1                   | ab                 | -       |

*table continues in next page...*

| Field | ID                   | <i>R</i><br>mag | <i>B</i><br>mag | redshift | redshift<br>quality | type of<br>spectra | EW[OII] |
|-------|----------------------|-----------------|-----------------|----------|---------------------|--------------------|---------|
| A963  | IJ101547.88+391435.9 | 19.04           | 21.12           | 0.2447   | 1                   | ab                 | –       |
| A963  | IJ101548.46+390433.9 | 18.33           | 20.33           | 0.1632   | 1                   | ab                 | –       |
| A963  | IJ101548.72+384414.8 | 18.78           | 21.05           | 0.2897   | -1                  | ab/em              | 5.61    |
| A963  | IJ101548.75+390420.1 | 19.32           | 20.79           | 0.1633   | 1                   | em+ab              | 15.52   |
| A963  | IJ101550.02+385903.0 | 18.77           | 21.07           | 0.2053   | 1                   | ab/em              | 6.52    |
| A963  | IJ101550.35+391543.3 | 17.80           | 20.14           | 0.2445   | 1                   | ab                 | –       |
| A963  | IJ101550.37+391117.2 | 18.70           | 20.65           | 0.2043   | 1                   | ab                 | –       |
| A963  | IJ101551.82+392030.6 | 17.88           | 19.19           | 0.2004   | -2                  | nan                | –       |
| A963  | IJ101552.14+390114.9 | 15.55           | 17.26           | 0.0629   | 1                   | ab/em              | 9.8     |
| A963  | IJ101554.56+390211.8 | 18.50           | 20.85           | 0.2002   | -2                  | nan                | –       |
| A963  | IJ101556.28+390326.0 | 18.85           | 20.32           | 0.2916   | 1                   | em/ab              | 7.7     |
| A963  | IJ101556.34+392002.9 | 17.63           | 19.16           | 0.2506   | -2                  | nan                | –       |
| A963  | IJ101559.23+391101.4 | 18.10           | 20.10           | 0.1393   | 1                   | ab                 | –       |
| A963  | IJ101559.50+384720.9 | 18.66           | 20.92           | 0.2712   | -2                  | nan                | –       |
| A963  | IJ101559.97+385445.9 | 18.80           | 20.77           | 0.1371   | -2                  | nan                | –       |
| A963  | IJ101600.06+391722.9 | 18.85           | 20.06           | 0.141    | 1                   | em                 | 82.05   |
| A963  | IJ101601.04+384434.5 | 18.70           | 21.10           | 0.2908   | 1                   | ab                 | –       |
| A963  | IJ101601.58+385452.4 | 17.96           | 19.42           | 0.1651   | 1                   | em+ab              | 10.77   |
| A963  | IJ101602.36+384759.4 | 19.33           | 21.07           | 0.2886   | -2                  | nan                | –       |
| A963  | IJ101604.55+384638.7 | 18.82           | 20.46           | 0.2001   | 1                   | ab/em              | 11.07   |
| A963  | IJ101606.44+391441.9 | 19.43           | 21.67           | 0.2201   | -1                  | ab                 | –       |
| A963  | IJ101606.60+392229.3 | 18.21           | 19.63           | 0.1626   | -1                  | ab                 | –       |
| A963  | IJ101607.65+384917.0 | 18.76           | 20.27           | 0.168    | 1                   | em/ab              | 21.68   |
| A963  | IJ101608.26+390012.9 | 18.87           | 21.15           | 0.2222   | 1                   | ab                 | –       |
| A963  | IJ101608.63+391016.9 | 17.63           | 19.84           | 0.2023   | 1                   | ab                 | –       |
| A963  | IJ101609.59+385004.4 | 18.51           | 19.90           | 0.1202   | 1                   | em+ab              | 26.69   |
| A963  | IJ101610.29+390725.0 | 19.03           | 21.04           | 0.2018   | 1                   | ab                 | –       |
| A963  | IJ101611.41+390204.0 | 19.32           | 20.90           | 0.2121   | -2                  | nan                | –       |
| A963  | IJ101612.16+384202.9 | 19.08           | 20.66           | 0.238    | 1                   | ab                 | –       |
| A963  | IJ101612.85+391647.9 | 18.08           | 19.24           | 0.0552   | 1                   | em                 | 47.05   |
| A963  | IJ101614.39+390411.1 | 18.13           | 19.36           | 0.097    | 1                   | em                 | 47.7    |
| A963  | IJ101614.75+385943.3 | 18.27           | 20.37           | 0.1681   | 1                   | ab                 | –       |
| A963  | IJ101614.77+384849.8 | 19.20           | 21.17           | 0.293    | -2                  | nan                | –       |
| A963  | IJ101618.05+390613.7 | 18.29           | 20.15           | 0.2076   | 1                   | ab/em              | 7.74    |
| A963  | IJ101621.01+384454.6 | 19.48           | 21.42           | 0.206    | -1                  | ab                 | –       |
| A963  | IJ101621.07+384256.7 | 17.96           | 20.27           | 0.2011   | 1                   | em+ab              | 18.55   |
| A963  | IJ101622.09+390225.0 | 17.56           | 18.92           | 0.2776   | 1                   | ab                 | –       |
| A963  | IJ101622.28+384912.9 | 17.77           | 20.09           | 0.2043   | 1                   | ab/em              | 12.1    |
| A963  | IJ101622.88+385903.8 | 16.98           | 19.17           | 0.1673   | 1                   | ab                 | –       |
| A963  | IJ101622.88+391853.0 | 18.46           | 20.83           | 0.1903   | 1                   | ab/em              | 11.81   |
| A963  | IJ101623.74+384501.0 | 18.43           | 20.68           | 0.1422   | 1                   | em+ab              | 45.06   |
| A963  | IJ101623.98+385840.4 | 18.28           | 20.41           | 0.1678   | 1                   | em+ab              | 23.58   |
| A963  | IJ101624.94+391251.9 | 18.76           | 20.81           | 0.2651   | 1                   | em+ab              | 5.38    |
| A963  | IJ101624.93+392020.6 | 19.48           | 21.84           | 0.395    | -1                  | ab                 | –       |
| A963  | IJ101625.29+390505.6 | 19.08           | 21.12           | 0.3766   | 1                   | em+ab              | 9.46    |
| A963  | IJ101625.49+390853.3 | 17.95           | 19.93           | 0.2098   | 1                   | ab                 | –       |
| A963  | IJ101625.87+385724.3 | 18.54           | 20.01           | 0.1452   | -1                  | em+ab              | 8.03    |
| A963  | IJ101626.34+385344.5 | 17.47           | 19.76           | 0.2016   | 1                   | ab                 | –       |
| A963  | IJ101627.02+384352.2 | 18.50           | 20.64           | 0.2565   | 1                   | ab                 | –       |
| A963  | IJ101629.57+384010.2 | 19.12           | 20.52           | 0.2029   | 1                   | ab                 | –       |
| A963  | IJ101630.23+390143.5 | 19.51           | 21.87           | 0.2078   | 1                   | ab                 | –       |
| A963  | IJ101631.76+391955.8 | 18.49           | 20.71           | 0.2038   | 1                   | ab                 | –       |
| A963  | IJ101631.97+392352.2 | 19.34           | 20.42           | 0.2371   | 1                   | em                 | 106.38  |
| A963  | IJ101633.80+390107.9 | 18.12           | 20.27           | 0.1992   | -1                  | ab                 | –       |
| A963  | IJ101633.81+384609.1 | 16.36           | 18.73           | 0.202    | 1                   | ab                 | –       |
| A963  | IJ101637.63+392021.6 | 17.54           | 19.75           | 0.2191   | 1                   | em                 | 20.78   |
| A963  | IJ101638.00+391935.4 | 18.31           | 20.53           | 0.2177   | 1                   | ab                 | –       |
| A963  | IJ101638.40+390623.3 | 19.51           | 21.39           | 0.3      | -2                  | nan                | –       |

*table continues in next page...*

| Field | ID                   | <i>R</i><br>mag | <i>B</i><br>mag | redshift | redshift<br>quality | type of<br>spectra | EW[OII] |
|-------|----------------------|-----------------|-----------------|----------|---------------------|--------------------|---------|
| A963  | IJ101638.42+392149.7 | 18.17           | 20.48           | 0.2083   | -1                  | ab                 | –       |
| A963  | IJ101638.84+384944.5 | 18.33           | 20.58           | 0.2031   | 1                   | ab                 | –       |
| A963  | IJ101639.07+390241.0 | 19.10           | 21.03           | 0.2053   | -2                  | nan                | –       |
| A963  | IJ101639.36+391836.4 | 19.51           | 20.72           | 0.1306   | 1                   | em                 | 17.88   |
| A963  | IJ101639.95+391438.7 | 18.47           | 20.74           | 0.2016   | -1                  | em+ab              | 17.35   |
| A963  | IJ101640.26+385713.7 | 18.52           | 20.82           | 0.202    | 1                   | ab                 | –       |
| A963  | IJ101640.29+384458.0 | 17.64           | 20.00           | 0.2027   | 1                   | ab                 | –       |
| A963  | IJ101640.96+385450.0 | 17.05           | 19.34           | 0.1993   | 1                   | ab                 | –       |
| A963  | IJ101642.98+384743.9 | 18.21           | 20.16           | 0.1211   | 1                   | ab/em              | 16.06   |
| A963  | IJ101644.42+390132.9 | 17.84           | 20.03           | 0.2049   | 1                   | ab                 | –       |
| A963  | IJ101645.06+384050.4 | 18.09           | 20.35           | 0.1997   | -1                  | ab                 | –       |
| A963  | IJ101646.02+384432.6 | 19.01           | 21.27           | 0.2691   | 1                   | ab/em              | 1.52    |
| A963  | IJ101646.46+384450.1 | 19.12           | 21.28           | 0.1272   | -1                  | em                 | 19.53   |
| A963  | IJ101646.47+385245.9 | 19.22           | 21.32           | 0.2024   | -1                  | ab                 | –       |
| A963  | IJ101646.72+385002.8 | 20.81           | 22.37           | 0.2824   | 1                   | ab                 | –       |
| A963  | IJ101646.74+385749.6 | 17.96           | 20.23           | 0.2041   | 1                   | ab                 | –       |
| A963  | IJ101647.50+384046.7 | 17.94           | 19.28           | 0.154    | 1                   | em                 | 46.13   |
| A963  | IJ101647.75+384128.6 | 18.78           | 20.63           | 0.1603   | -2                  | nan                | –       |
| A963  | IJ101649.69+390215.6 | 18.22           | 20.35           | 0.2025   | -1                  | ab                 | –       |
| A963  | IJ101652.09+392209.4 | 17.91           | 20.14           | 0.2054   | 1                   | ab                 | –       |
| A963  | IJ101652.27+391101.4 | 18.43           | 19.95           | 0.1555   | 1                   | em+ab              | 18.0    |
| A963  | IJ101652.64+385657.4 | 18.49           | 20.65           | 0.1973   | 1                   | ab                 | –       |
| A963  | IJ101652.87+385544.7 | 19.23           | 21.16           | 0.2025   | 1                   | ab                 | –       |
| A963  | IJ101652.96+383906.1 | 19.37           | 20.69           | 0.1551   | 1                   | em/ab              | 164.3   |
| A963  | IJ101653.25+384325.8 | 17.60           | 19.62           | 0.1994   | 1                   | ab/em              | 3.32    |
| A963  | IJ101653.43+391331.6 | 18.95           | 21.14           | 0.2033   | 1                   | ab                 | –       |
| A963  | IJ101654.39+391843.8 | 18.95           | 21.11           | 0.2066   | -2                  | nan                | –       |
| A963  | IJ101654.86+390823.0 | 17.62           | 18.82           | 0.1302   | 1                   | em/ab              | 10.75   |
| A963  | IJ101656.78+385656.2 | 17.59           | 19.84           | 0.2048   | 1                   | ab                 | –       |
| A963  | IJ101657.32+391948.4 | 18.23           | 20.42           | 0.1966   | -1                  | ab                 | –       |
| A963  | IJ101657.74+392100.8 | 18.51           | 20.80           | 0.2075   | -1                  | ab                 | –       |
| A963  | IJ101659.58+384956.2 | 18.80           | 20.86           | 0.2066   | -1                  | ab                 | –       |
| A963  | IJ101659.77+392159.7 | 17.97           | 19.25           | 0.2348   | 1                   | ab                 | –       |
| A963  | IJ101701.26+390040.9 | 19.18           | 21.48           | 0.2059   | 1                   | ab                 | –       |
| A963  | IJ101702.70+390132.5 | 18.14           | 20.47           | 0.2146   | 1                   | ab                 | –       |
| A963  | IJ101703.47+384157.7 | 18.42           | 20.35           | 0.2451   | -2                  | nan                | –       |
| A963  | IJ101703.50+385052.8 | 18.48           | 20.75           | 0.1969   | 1                   | ab                 | –       |
| A963  | IJ101703.71+391618.8 | 16.82           | 19.10           | 0.2071   | 1                   | ab                 | –       |
| A963  | IJ101703.95+391754.3 | 17.54           | 19.81           | 0.1741   | -1                  | ab                 | –       |
| A963  | IJ101704.15+391249.4 | 19.15           | 21.42           | 0.2046   | 1                   | ab                 | –       |
| A963  | IJ101704.41+385948.1 | 18.25           | 20.58           | 0.2087   | 1                   | ab                 | –       |
| A963  | IJ101704.50+385542.1 | 18.29           | 20.32           | 0.169    | -2                  | nan                | –       |
| A963  | IJ101705.77+384630.1 | 17.86           | 20.20           | 0.2      | 1                   | ab                 | –       |
| A963  | IJ101705.77+390815.5 | 17.31           | 18.97           | 0.2054   | -2                  | nan                | –       |
| A963  | IJ101705.95+385029.0 | 17.90           | 19.02           | 0.0673   | 1                   | em                 | 46.83   |
| A963  | IJ101706.86+391921.0 | 18.47           | 20.50           | 0.2071   | 1                   | ab                 | –       |
| A963  | IJ101707.14+391703.0 | 18.78           | 21.13           | 0.2707   | -2                  | nan                | –       |
| A963  | IJ101707.31+385626.5 | 18.28           | 20.10           | 0.201    | 1                   | ab/em              | 7.57    |
| A963  | IJ101707.36+390338.5 | 17.24           | 19.56           | 0.2058   | 1                   | ab                 | –       |
| A963  | IJ101707.44+384228.0 | 18.46           | 20.76           | 0.282    | -2                  | nan                | –       |
| A963  | IJ101707.45+390425.2 | 18.24           | 20.01           | 0.2113   | 1                   | em+ab              | 4.3     |
| A963  | IJ101708.31+390116.2 | 19.39           | 21.68           | 0.1411   | -2                  | nan                | –       |
| A963  | IJ101708.31+385242.7 | 18.91           | 21.22           | 0.2943   | -1                  | ab/em              | 6.49    |
| A963  | IJ101709.08+384805.3 | 19.10           | 20.87           | 0.2709   | -2                  | nan                | –       |
| A963  | IJ101710.93+384318.5 | 19.49           | 20.92           | 0.2036   | 1                   | em/ab              | 51.77   |
| A963  | IJ101711.03+390310.6 | 18.45           | 20.67           | 0.154    | -1                  | em                 | 25.06   |
| A963  | IJ101711.34+383807.7 | 19.48           | 21.77           | 0.1642   | -2                  | nan                | –       |
| A963  | IJ101712.21+390559.3 | 18.33           | 19.68           | 0.1644   | 1                   | em                 | 57.3    |

*table continues in next page...*

| Field | ID                   | <i>R</i><br>mag | <i>B</i><br>mag | redshift | redshift<br>quality | type of<br>spectra | EW[OII] |
|-------|----------------------|-----------------|-----------------|----------|---------------------|--------------------|---------|
| A963  | IJ101713.88+390131.7 | 17.92           | 20.18           | 0.221    | -2                  | nan                | –       |
| A963  | IJ101713.89+391040.2 | 19.12           | 21.23           | 0.3176   | -2                  | nan                | –       |
| A963  | IJ101714.13+385955.4 | 18.20           | 20.41           | 0.2026   | 1                   | ab                 | –       |
| A963  | IJ101714.88+390551.6 | 17.92           | 19.32           | 0.1639   | 1                   | em+ab              | 13.06   |
| A963  | IJ101715.02+384820.8 | 18.02           | 20.23           | 0.2021   | 1                   | ab                 | –       |
| A963  | IJ101715.30+383712.2 | 19.17           | 20.60           | 0.24     | 1                   | em+ab              | 7.88    |
| A963  | IJ101715.54+385011.9 | 17.52           | 19.83           | 0.1976   | 1                   | ab/em              | 5.17    |
| A963  | IJ101715.62+391248.1 | 18.45           | 20.84           | 0.2891   | -1                  | nan                | –       |
| A963  | IJ101716.03+391259.5 | 18.23           | 20.30           | 0.2122   | -2                  | nan                | –       |
| A963  | IJ101716.96+390206.0 | 19.43           | 20.79           | 0.2004   | 1                   | em                 | 11.96   |
| A963  | IJ101717.00+391300.8 | 19.21           | 21.58           | 0.2997   | 1                   | ab                 | –       |
| A963  | IJ101717.01+384839.9 | 18.04           | 19.68           | 0.0884   | 1                   | em+ab              | 13.55   |
| A963  | IJ101717.14+385916.6 | 18.29           | 20.48           | 0.2038   | 1                   | ab                 | –       |
| A963  | IJ101717.44+390120.2 | 18.10           | 20.46           | 0.2053   | -1                  | ab                 | –       |
| A963  | IJ101720.10+390607.3 | 17.93           | 19.67           | 0.1651   | 1                   | em+ab              | 17.31   |
| A963  | IJ101720.23+385534.1 | 18.91           | 21.12           | 0.2043   | 1                   | ab                 | –       |
| A963  | IJ101721.48+391408.2 | 19.16           | 20.73           | 0.2682   | -1                  | em+ab              | 32.75   |
| A963  | IJ101722.03+390439.9 | 16.89           | 19.19           | 0.1973   | 1                   | ab                 | –       |
| A963  | IJ101722.08+390153.8 | 19.02           | 20.41           | 0.1989   | 1                   | em+ab              | 15.44   |
| A963  | IJ101722.09+385839.3 | 17.66           | 19.71           | 0.1478   | 1                   | ab                 | –       |
| A963  | IJ101722.18+390007.1 | 16.87           | 19.07           | 0.1983   | 1                   | ab                 | –       |
| A963  | IJ101722.64+390431.8 | 18.22           | 20.53           | 0.4058   | -1                  | em                 | 4.24    |
| A963  | IJ101723.25+383702.2 | 19.06           | 21.34           | 0.2877   | -1                  | em                 | 19.69   |
| A963  | IJ101724.84+385533.4 | 17.95           | 19.65           | 0.1493   | 1                   | ab                 | –       |
| A963  | IJ101725.74+391328.4 | 19.31           | 21.26           | 0.2063   | -1                  | ab/em              | 4.79    |
| A963  | IJ101726.38+385941.4 | 18.80           | 20.97           | 0.2085   | 1                   | ab                 | –       |
| A963  | IJ101726.41+390432.8 | 17.35           | 19.72           | 0.21     | 1                   | ab/em              | 16.83   |
| A963  | IJ101726.48+391846.0 | 19.29           | 21.65           | 0.3      | -1                  | ab                 | –       |
| A963  | IJ101728.07+385952.7 | 19.75           | 20.93           | 0.1991   | 1                   | em                 | 18.71   |
| A963  | IJ101730.57+385342.8 | 18.52           | 20.41           | 0.2935   | 1                   | ab/em              | 6.49    |
| A963  | IJ101731.25+392300.7 | 18.10           | 20.51           | 0.21     | -1                  | em                 | 36.5    |
| A963  | IJ101732.36+390114.5 | 18.42           | 20.66           | 0.202    | 1                   | em                 | 48.9    |
| A963  | IJ101735.37+392237.8 | 18.49           | 20.01           | 0.2701   | 1                   | em                 | 23.86   |
| A963  | IJ101736.01+384148.9 | 19.30           | 21.25           | 0.2421   | 1                   | em/ab              | 19.45   |
| A963  | IJ101736.61+391716.3 | 18.79           | 20.62           | 0.3001   | -2                  | nan                | –       |
| A963  | IJ101738.22+383714.7 | 18.83           | 20.67           | 0.1108   | -2                  | nan                | –       |
| A963  | IJ101738.27+384257.3 | 17.83           | 19.80           | 0.168    | -1                  | ab                 | –       |
| A963  | IJ101739.46+385630.3 | 18.89           | 20.82           | 0.3469   | -1                  | ab/em              | 3.42    |
| A963  | IJ101740.16+384147.8 | 18.12           | 19.94           | 0.249    | -2                  | nan                | –       |
| A963  | IJ101743.43+392528.9 | 19.43           | 21.45           | 0.1138   | -1                  | ab                 | –       |
| A963  | IJ101743.89+385629.3 | 18.31           | 20.27           | 0.1244   | 1                   | em/ab              | 13.66   |
| A963  | IJ101747.58+384427.9 | 19.45           | 21.19           | 0.2679   | 1                   | em+ab              | 11.89   |
| A963  | IJ101747.72+392313.4 | 18.09           | 19.43           | 0.1006   | -2                  | nan                | –       |
| A963  | IJ101751.19+392517.2 | 19.06           | 20.45           | 0.1886   | 1                   | em/ab              | 33.69   |
| A963  | IJ101751.86+383901.0 | 17.93           | 19.93           | 0.176    | -2                  | nan                | –       |
| A963  | IJ101752.16+383816.0 | 17.45           | 19.66           | 0.2167   | -2                  | nan                | –       |
| A963  | IJ101752.92+392235.6 | 19.05           | 20.69           | 0.1589   | -2                  | nan                | –       |
| A963  | IJ101753.96+391356.6 | 17.97           | 20.14           | 0.2584   | -1                  | em                 | –       |
| A963  | IJ101758.42+392333.2 | 18.36           | 20.33           | 0.2013   | 1                   | em/ab              | 18.33   |
| A963  | IJ101800.18+385834.2 | 19.16           | 21.29           | 0.1298   | -2                  | nan                | –       |
| A963  | IJ101801.00+391705.8 | 19.02           | 20.84           | 0.3054   | 1                   | em+ab              | 8.32    |
| A963  | IJ101801.52+391246.9 | 18.92           | 20.70           | 0.295    | 1                   | em/ab              | 26.27   |
| A963  | IJ101802.96+390745.0 | 18.41           | 20.26           | 0.2189   | -1                  | ab                 | –       |
| A963  | IJ101805.29+392350.1 | 18.14           | 19.42           | 0.1492   | 1                   | em                 | 25.78   |
| A963  | IJ101805.95+385756.2 | 18.51           | 20.11           | 0.3679   | 1                   | em                 | 43.2    |
| A963  | IJ101808.84+385540.5 | 18.00           | 19.66           | 0.2031   | 1                   | em+ab              | 8.6     |
| A963  | IJ101813.36+390510.3 | 18.36           | 20.55           | 0.2979   | 1                   | ab                 | –       |
| A963  | IJ101814.48+390221.2 | 18.25           | 19.36           | 0.2739   | -1                  | ab                 | –       |

*table continues in next page...*

| Field | ID                   | <i>R</i><br>mag | <i>B</i><br>mag | redshift | redshift<br>quality | type of<br>spectra | EW[OII] |
|-------|----------------------|-----------------|-----------------|----------|---------------------|--------------------|---------|
| A963  | IJ101814.66+385418.9 | 19.26           | 21.45           | 0.2036   | -1                  | ab                 | –       |
| A963  | IJ101820.58+390410.1 | 16.85           | 19.21           | 0.2188   | -1                  | ab                 | –       |
| A963  | IJ101823.19+391042.6 | 17.86           | 19.77           | 0.1479   | 1                   | ab                 | –       |
| A963  | IJ101823.63+391104.3 | 18.86           | 20.20           | 0.2392   | 1                   | em                 | 27.27   |
| A963  | IJ101824.59+390414.7 | 19.04           | 21.09           | 0.2898   | -1                  | ab                 | –       |
| A963  | IJ101825.19+385740.1 | 19.25           | 21.45           | 0.3893   | 1                   | ab/em              | 6.68    |
| A963  | IJ101827.04+384211.7 | 19.04           | 21.23           | 0.202    | -1                  | ab                 | –       |
| A963  | IJ101829.15+390905.8 | 18.01           | 19.53           | 0.1554   | -1                  | ab                 | –       |
| A963  | IJ101832.79+385828.2 | 19.48           | 21.19           | 0.3773   | 1                   | em                 | 15.74   |
| A963  | IJ101833.17+385525.1 | 19.51           | 21.08           | 0.2161   | 1                   | ab/em              | 9.05    |
| A963  | IJ101833.63+385422.2 | 17.98           | 19.63           | 0.2478   | 1                   | em+ab              | 8.83    |
| A963  | IJ101833.72+391312.8 | 19.20           | 21.15           | 0.1569   | -1                  | ab                 | –       |
| A963  | IJ101835.03+390232.0 | 18.53           | 19.93           | 0.1395   | 1                   | em+ab              | 12.75   |
| A963  | IJ101837.07+390805.7 | 18.62           | 20.47           | 0.3757   | -1                  | ab/em              | 4.17    |
| A963  | IJ101837.26+385235.1 | 19.03           | 20.96           | 0.2028   | 1                   | ab/em              | 8.63    |
| A963  | IJ101839.58+385333.9 | 18.19           | 20.35           | 0.2009   | 1                   | em+ab              | 15.72   |
| A963  | IJ101840.86+385017.8 | 17.59           | 19.86           | 0.2389   | 1                   | ab                 | –       |
| A963  | IJ101843.83+391506.4 | 18.00           | 20.06           | 0.1481   | 1                   | ab                 | –       |
| A963  | IJ101846.16+391149.7 | 18.54           | 20.50           | 0.2582   | 1                   | em+ab              | 6.33    |
| A963  | IJ101846.20+391100.8 | 17.69           | 18.82           | 0.1548   | -2                  | nan                | –       |
| A963  | IJ101848.40+391526.7 | 16.93           | 18.93           | 0.1469   | 1                   | ab+em              | –       |
| A963  | IJ101850.03+391707.4 | 19.13           | 20.80           | 0.1688   | -2                  | nan                | –       |
| A963  | IJ101850.72+384746.2 | 17.72           | 19.74           | 0.1486   | 1                   | ab                 | –       |
| A963  | IJ101850.93+384926.0 | 17.57           | 19.52           | 0.1611   | -1                  | ab                 | –       |
| A963  | IJ101851.89+391312.5 | 17.61           | 18.80           | 0.1049   | 1                   | em/ab              | 36.79   |
| A963  | IJ101853.54+391517.5 | 17.44           | 19.45           | 0.0638   | 1                   | em                 | 64.21   |
| A963  | IJ101853.92+384803.0 | 19.32           | 20.73           | 0.2171   | 1                   | em                 | 28.07   |
| A963  | IJ101855.92+385412.7 | 18.50           | 20.52           | 0.2184   | 1                   | em/ab              | 13.3    |
| A963  | IJ101856.31+385414.9 | 18.60           | 20.73           | 0.217    | -1                  | ab                 | –       |
| A963  | IJ101856.71+390158.5 | 17.78           | 19.56           | 0.1596   | 1                   | em                 | 8.7     |
| A963  | IJ101859.19+385916.5 | 18.96           | 20.56           | 0.3629   | -2                  | nan                | –       |
| A963  | IJ101859.61+391012.7 | 18.52           | 20.53           | 0.1483   | -2                  | nan                | –       |
| A963  | IJ101900.28+385427.8 | 18.29           | 20.61           | 0.2176   | 1                   | ab                 | –       |
| A963  | IJ101901.04+391032.1 | 19.25           | 20.59           | 0.2051   | 1                   | em+ab              | 38.35   |
| A963  | IJ101902.26+391042.4 | 18.15           | 19.94           | 0.1467   | 1                   | ab+em              | –       |
| A963  | IJ101908.87+385023.5 | 19.46           | 21.42           | 0.3598   | 1                   | em+ab              | 25.3    |
| A963  | IJ101909.06+390506.6 | 19.11           | 20.38           | 0.1627   | 1                   | em+ab              | 23.39   |
| A963  | IJ101913.03+390136.0 | 18.89           | 21.30           | 0.3773   | 1                   | ab                 | –       |
| A963  | IJ101915.04+385708.5 | 18.01           | 19.39           | 0.1115   | 1                   | em                 | 29.27   |
| A963  | IJ101916.12+390426.4 | 18.42           | 20.54           | 0.0799   | 1                   | nan                | –       |
| A963  | IJ101916.92+385824.9 | 19.42           | 21.10           | 0.1608   | 1                   | em                 | 43.98   |
| A963  | IJ101519.02+390647.2 | 18.10           | 19.68           | 0.454    | -1                  | ab                 | –       |
| A963  | IJ101747.24+384227.8 | 17.79           | 19.78           | 0.3043   | -1                  | ab                 | –       |
| A963  | IJ101847.29+391734.6 | 17.24           | 19.38           | 0.2378   | -2                  | nan                | –       |
| A963  | IJ101841.41+391934.3 | 17.53           | 19.59           | 0.2117   | -2                  | nan                | –       |
| A963  | IJ101547.33+385246.6 | 18.02           | 20.10           | 0.1682   | -2                  | nan                | –       |
| A963  | IJ101701.24+390502.0 | 19.23           | 21.48           | 0.3058   | -1                  | ab                 | –       |
| A963  | IJ101837.12+390708.1 | 18.84           | 19.96           | 0.1705   | -1                  | ab                 | –       |
| A963  | IJ101707.44+390903.9 | 19.02           | 20.08           | 0.2032   | -2                  | nan                | –       |
| A963  | IJ101828.74+390609.3 | 19.11           | 20.19           | 0.1247   | 1                   | em+ab              | 24.48   |
| A963  | IJ101829.70+390725.2 | 19.13           | 20.25           | 0.1394   | 1                   | em+ab              | 12.14   |
| A963  | IJ101848.66+391757.1 | 18.53           | 20.85           | 0.261    | 1                   | ab                 | –       |
| A963  | IJ101550.60+385350.7 | 18.55           | 20.69           | 0.1435   | -2                  | nan                | –       |
| A963  | IJ101803.64+384120.8 | 17.75           | 19.35           | 0.2056   | 1                   | em+ab              | 10.99   |
| A963  | IJ101727.09+384144.1 | 18.01           | 19.74           | 0.2066   | -1                  | ab                 | –       |
| A963  | IJ101756.27+383807.9 | 18.90           | 19.96           | 0.205    | 1                   | em/ab              | 38.59   |
| A963  | IJ101536.22+384533.1 | 18.62           | 19.81           | 0.2056   | 1                   | em/ab              | 37.46   |
| A963  | IJ101600.12+385205.9 | 20.14           | 21.27           | 0.2087   | 1                   | em                 | 26.43   |

*table continues in next page...*

| Field | ID                   | <i>R</i><br>mag | <i>B</i><br>mag | redshift | redshift<br>quality | type of<br>spectra | EW[OII] |
|-------|----------------------|-----------------|-----------------|----------|---------------------|--------------------|---------|
| A963  | IJ101606.49+385118.6 | 19.78           | 21.51           | 0.2688   | -1                  | ab                 | –       |
| A963  | IJ101613.96+385122.8 | 19.71           | 21.14           | 0.2071   | 1                   | em                 | 57.73   |
| A963  | IJ101611.14+384924.7 | 17.43           | 19.28           | 0.206    | 1                   | nan                | –       |
| A963  | IJ101636.11+384434.5 | 19.51           | 20.94           | 0.2077   | 1                   | em                 | 20.37   |
| A963  | IJ101749.47+385400.8 | 20.57           | 21.81           | 0.2071   | -1                  | em+a               | 20.56   |
| A963  | IJ101731.90+385401.8 | 19.45           | 20.78           | 0.2156   | 1                   | em/ab              | 28.45   |
| A963  | IJ101742.99+384950.1 | 20.75           | 21.80           | 0.2067   | 1                   | em                 | 77.11   |
| A963  | IJ101719.92+384608.9 | 19.54           | 20.93           | 0.2062   | 1                   | em/ab              | 31.07   |
| A963  | IJ101701.12+384259.6 | 19.35           | 20.73           | 0.2033   | 1                   | em                 | 23.32   |
| A963  | IJ101705.48+384925.5 | 18.40           | 20.11           | 0.2044   | 1                   | em+ab              | 16.08   |
| A963  | IJ101702.78+385115.7 | 19.73           | 21.32           | 0.2058   | -1                  | em/ab              | 23.0    |
| A963  | IJ101751.19+390923.3 | 19.95           | 21.08           | 0.1996   | 1                   | em/ab              | 35.62   |
| A963  | IJ101740.73+390734.1 | 19.19           | 20.34           | 0.2086   | 1                   | em                 | 27.53   |
| A963  | IJ101734.63+391354.0 | 19.72           | 21.06           | 0.2179   | 1                   | em                 | 14.94   |
| A963  | IJ101717.54+391334.9 | 19.31           | 20.38           | 0.2106   | 1                   | em                 | 43.42   |
| A963  | IJ101709.08+391136.8 | 19.79           | 21.13           | 0.2183   | -2                  | nan                | –       |
| A963  | IJ101709.18+391800.9 | 20.55           | 21.73           | 0.219    | -2                  | nan                | –       |
| A963  | IJ101645.42+391941.0 | 19.25           | 20.85           | 0.1688   | 1                   | em                 | 41.3    |
| A963  | IJ101626.35+391901.3 | 19.16           | 21.09           | 0.2191   | -1                  | ab                 | –       |
| A963  | IJ101629.18+391256.4 | 18.01           | 19.37           | 0.2102   | 1                   | em/ab              | 34.32   |
| A963  | IJ101641.11+391026.1 | 18.84           | 20.05           | 0.2103   | 1                   | em                 | 35.27   |
| A963  | IJ101646.92+390901.5 | 20.02           | 21.09           | 0.2097   | 1                   | em/ab              | 21.39   |
| A963  | IJ101644.50+390745.0 | 19.58           | 21.08           | 0.2078   | 1                   | em                 | 21.13   |
| A963  | IJ101625.04+391101.6 | 19.20           | 20.36           | 0.1675   | 1                   | em                 | 46.82   |
| A963  | IJ101628.19+390931.9 | 17.78           | 19.14           | 0.2104   | 1                   | em+ab              | 20.26   |
| A963  | IJ101621.18+390758.4 | 20.05           | 21.21           | 0.2067   | 1                   | em                 | 52.89   |
| A963  | IJ101627.95+390457.9 | 19.22           | 20.40           | 0.1653   | 1                   | em                 | 37.77   |
| A963  | IJ101846.29+385915.8 | 18.65           | 20.12           | 0.2016   | 1                   | em+ab              | 4.74    |
| A963  | IJ101835.21+385817.7 | 17.94           | 19.72           | 0.3216   | -2                  | nan                | –       |
| A963  | IJ101820.00+390010.2 | 18.85           | 20.22           | 0.2059   | 1                   | em                 | 19.17   |
| A963  | IJ101833.28+390357.0 | 17.75           | 19.25           | 0.2986   | -2                  | nan                | –       |
| A963  | IJ101809.28+390717.1 | 18.92           | 20.41           | 0.2076   | -1                  | em                 | 20.46   |
| A963  | IJ101759.81+390239.1 | 20.58           | 21.94           | 0.2749   | -2                  | nan                | –       |
| A963  | IJ101752.32+390111.6 | 20.46           | 21.62           | 0.2026   | 1                   | em                 | 31.6    |
| A963  | IJ101642.81+390136.1 | 18.69           | 19.77           | 0.165    | 1                   | em                 | 39.42   |
| A963  | IJ101642.35+385900.8 | 19.20           | 20.43           | 0.1688   | 1                   | em/ab              | 61.95   |
| A963  | IJ101744.58+390446.8 | 19.53           | 20.80           | 0.2005   | 1                   | em/ab              | 30.64   |
| A963  | IJ101730.00+385831.1 | 19.40           | 20.99           | 0.2041   | 1                   | em+ab              | 32.51   |
| A963  | IJ101719.40+385834.3 | 20.07           | 21.26           | 0.2181   | -1                  | em                 | 33.12   |
| A963  | IJ101701.54+390009.3 | 19.78           | 20.89           | 0.1649   | 1                   | em                 | 57.22   |
| A963  | IJ101719.63+390556.9 | 19.85           | 21.04           | 0.2101   | 1                   | em                 | 17.93   |
| A963  | IJ101739.17+390346.4 | 19.86           | 21.03           | 0.2002   | 1                   | em                 | 25.65   |
| A963  | IJ101725.90+390522.4 | 19.70           | 20.77           | 0.1693   | 1                   | em                 | 34.9    |
| A963  | IJ101729.04+390403.5 | 17.68           | 18.81           | 0.1695   | 1                   | em+ab              | 24.37   |
| A963  | IJ101618.24+384255.3 | 18.41           | 19.88           | 0.2011   | 1                   | em                 | 26.35   |
| A963  | IJ101727.74+384628.6 | 18.52           | 20.09           | 0.2011   | 1                   | em/ab              | 44.38   |
| A963  | IJ101624.27+390742.5 | 20.27           | 21.41           | 0.202    | 1                   | em+ab              | 32.65   |
| A963  | IJ101806.13+390753.8 | 18.73           | 20.48           | 0.1262   | -2                  | nan                | –       |
| A963  | IJ101743.02+390105.9 | 19.44           | 21.30           | 0.2089   | 1                   | ab                 | –       |
| A2192 | IJ162431.50+424621.7 | 18.32           | 19.99           | 0.2612   | 1                   | ab                 | –       |
| A2192 | IJ162433.27+424202.9 | 18.70           | 20.27           | 0.261    | 1                   | em+ab              | 19.06   |
| A2192 | IJ162436.20+424111.7 | 19.00           | 20.96           | 0.1427   | -2                  | ab                 | –       |
| A2192 | IJ162436.24+424934.6 | 19.25           | 21.21           | 0.2594   | 1                   | em+ab              | 23.21   |
| A2192 | IJ162436.65+424459.0 | 19.29           | 20.85           | 0.1894   | 1                   | em                 | 39.51   |
| A2192 | IJ162438.09+424216.9 | 19.52           | 20.95           | 0.19     | 1                   | em                 | 21.36   |
| A2192 | IJ162444.17+424131.9 | 17.40           | 19.58           | 0.1881   | 1                   | ab                 | –       |

*table continues in next page...*

| Field | ID                   | <i>R</i><br>mag | <i>B</i><br>mag | redshift | redshift<br>quality | type of<br>spectra | EW[OII] |
|-------|----------------------|-----------------|-----------------|----------|---------------------|--------------------|---------|
| A2192 | IJ162448.24+422853.7 | 17.93           | 19.69           | 0.2315   | 1                   | em                 | 27.87   |
| A2192 | IJ162448.52+423222.8 | 18.04           | 19.91           | 0.1335   | 1                   | ab/em              | 2.38    |
| A2192 | IJ162449.35+424022.9 | 18.34           | 19.96           | 0.1592   | 1                   | ab                 | –       |
| A2192 | IJ162449.42+425012.5 | 19.50           | 21.03           | 0.2666   | 1                   | em+ab              | 36.44   |
| A2192 | IJ162451.50+422756.8 | 18.90           | 21.12           | 0.2316   | 1                   | ab                 | –       |
| A2192 | IJ162451.65+422828.9 | 20.01           | 20.99           | 0.1894   | 1                   | em/ab              | 90.67   |
| A2192 | IJ162451.96+425517.1 | 17.66           | 19.46           | 0.1895   | 1                   | ab                 | –       |
| A2192 | IJ162453.62+424558.4 | 19.19           | 21.43           | 0.2271   | 1                   | ab                 | –       |
| A2192 | IJ162454.48+424703.8 | 18.46           | 20.74           | 0.227    | 1                   | nan                | –       |
| A2192 | IJ162454.87+425603.5 | 19.50           | 21.42           | 0.1928   | 1                   | em+ab              | 107.54  |
| A2192 | IJ162456.26+425400.3 | 18.70           | 20.22           | 0.2602   | 1                   | em/ab              | 8.37    |
| A2192 | IJ162456.51+424010.6 | 18.73           | 20.48           | 0.26     | 1                   | em                 | 16.76   |
| A2192 | IJ162458.49+423306.8 | 18.74           | 20.71           | 0.2989   | 1                   | ab/em              | 17.2    |
| A2192 | IJ162459.62+423041.4 | 17.94           | 19.14           | 0.1299   | 1                   | em                 | 11.12   |
| A2192 | IJ162501.11+422348.0 | 19.10           | 20.74           | 0.3116   | 1                   | ab/em              | 16.29   |
| A2192 | IJ162503.93+423333.1 | 18.09           | 19.78           | 0.1349   | 1                   | em                 | 13.43   |
| A2192 | IJ162504.60+422818.4 | 19.15           | 20.84           | 0.2665   | 1                   | ab/em              | 6.22    |
| A2192 | IJ162504.66+424746.0 | 17.88           | 19.78           | 0.1866   | -2                  | nan                | –       |
| A2192 | IJ162506.34+423513.6 | 17.37           | 19.50           | 0.189    | 1                   | ab                 | –       |
| A2192 | IJ162506.38+425129.3 | 19.23           | 21.18           | 0.1866   | 1                   | ab                 | –       |
| A2192 | IJ162506.55+424750.4 | 19.21           | 20.99           | 0.2257   | 1                   | em                 | 9.95    |
| A2192 | IJ162506.82+425316.3 | 19.17           | 20.63           | 0.2253   | 1                   | em+ab              | 21.35   |
| A2192 | IJ162508.65+423400.9 | 18.10           | 19.57           | 0.1899   | 1                   | em                 | 8.17    |
| A2192 | IJ162509.08+424819.3 | 19.40           | 21.54           | 0.226    | -1                  | ab                 | –       |
| A2192 | IJ162509.77+425254.8 | 18.41           | 19.89           | 0.225    | 1                   | em                 | 13.94   |
| A2192 | IJ162510.10+423401.7 | 18.81           | 20.96           | 0.1867   | 1                   | em+ab              | 10.22   |
| A2192 | IJ162510.26+425051.8 | 17.91           | 19.46           | 0.2339   | 1                   | em                 | 11.27   |
| A2192 | IJ162510.60+424029.4 | 19.22           | 20.42           | 0.1875   | 1                   | em/ab              | 40.22   |
| A2192 | IJ162510.93+424823.0 | 17.72           | 19.98           | 0.225    | 1                   | ab                 | –       |
| A2192 | IJ162511.52+425605.6 | 19.43           | 20.47           | 0.2824   | -2                  | nan                | –       |
| A2192 | IJ162511.98+424218.9 | 18.98           | 20.98           | 0.2098   | 1                   | ab                 | –       |
| A2192 | IJ162512.54+425855.4 | 18.22           | 19.88           | 0.083    | -2                  | nan                | –       |
| A2192 | IJ162512.95+422741.1 | 19.41           | 21.52           | 0.2665   | 1                   | em                 | 15.53   |
| A2192 | IJ162513.52+423752.5 | 19.35           | 21.64           | 0.2366   | 1                   | ab                 | –       |
| A2192 | IJ162513.68+424832.9 | 18.68           | 20.88           | 0.227    | -2                  | nan                | –       |
| A2192 | IJ162518.02+422036.6 | 18.95           | 20.37           | 0.1587   | -1                  | em/ab              | 26.19   |
| A2192 | IJ162521.41+424156.4 | 19.17           | 21.25           | 0.1888   | 1                   | ab                 | –       |
| A2192 | IJ162523.68+422740.9 | 18.28           | 19.90           | 0.1869   | 1                   | em                 | 9.06    |
| A2192 | IJ162523.90+422208.6 | 19.30           | 20.42           | 0.1347   | 1                   | em                 | 38.31   |
| A2192 | IJ162523.95+422336.5 | 18.65           | 19.75           | 0.1963   | -1                  | ab                 | –       |
| A2192 | IJ162524.84+422002.8 | 18.69           | 19.68           | 0.2565   | -2                  | nan                | –       |
| A2192 | IJ162526.46+422728.7 | 18.74           | 20.44           | 0.2192   | 1                   | em+ab              | 8.46    |
| A2192 | IJ162528.43+424708.6 | 17.79           | 19.06           | 0.189    | 1                   | em                 | 28.63   |
| A2192 | IJ162531.14+424856.6 | 17.53           | 18.66           | 0.1586   | 1                   | ab                 | –       |
| A2192 | IJ162532.86+422344.8 | 18.97           | 20.21           | 0.1904   | 1                   | em/ab              | 17.83   |
| A2192 | IJ162533.73+424324.6 | 19.29           | 20.69           | 0.2508   | 1                   | em                 | 27.97   |
| A2192 | IJ162534.98+425500.9 | 18.56           | 20.51           | 0.2299   | 1                   | ab                 | –       |
| A2192 | IJ162536.19+424132.4 | 19.50           | 20.78           | 0.1902   | 1                   | em+ab              | 47.34   |
| A2192 | IJ162537.22+422756.4 | 19.42           | 20.94           | 0.3498   | 1                   | em/ab              | 20.09   |
| A2192 | IJ162538.12+422630.6 | 17.65           | 19.33           | 0.1581   | 1                   | ab                 | –       |
| A2192 | IJ162538.89+425055.6 | 19.12           | 21.25           | 0.2005   | 1                   | ab                 | –       |
| A2192 | IJ162539.32+422030.0 | 19.33           | 21.53           | 0.1378   | 1                   | nan                | –       |
| A2192 | IJ162539.48+423005.0 | 19.40           | 20.93           | 0.3927   | 1                   | em                 | 13.8    |
| A2192 | IJ162540.94+423942.0 | 18.82           | 20.85           | 0.1898   | 1                   | ab                 | –       |
| A2192 | IJ162541.64+430041.5 | 19.43           | 21.08           | 0.0945   | -1                  | em                 | 72.68   |
| A2192 | IJ162542.80+421717.2 | 18.65           | 20.53           | 0.2679   | 1                   | em/ab              | 16.54   |
| A2192 | IJ162544.40+424953.8 | 17.65           | 19.60           | 0.1679   | 1                   | ab                 | –       |
| A2192 | IJ162547.62+425125.4 | 18.28           | 20.39           | 0.2684   | 1                   | ab                 | –       |

*table continues in next page...*

| Field | ID                   | <i>R</i><br>mag | <i>B</i><br>mag | redshift | redshift<br>quality | type of<br>spectra | EW[OII] |
|-------|----------------------|-----------------|-----------------|----------|---------------------|--------------------|---------|
| A2192 | IJ162548.43+422632.7 | 18.48           | 19.53           | 0.1899   | 1                   | em                 | 35.37   |
| A2192 | IJ162549.32+424037.2 | 16.90           | 19.02           | 0.1898   | 1                   | em                 | 4.3     |
| A2192 | IJ162549.36+422316.2 | 17.79           | 19.88           | 0.1905   | 1                   | ab                 | –       |
| A2192 | IJ162550.34+422416.1 | 18.79           | 20.46           | 0.1898   | 1                   | em                 | 19.35   |
| A2192 | IJ162550.43+422156.0 | 19.24           | 20.85           | 0.1901   | 1                   | em/ab              | 8.77    |
| A2192 | IJ162550.81+423507.7 | 19.03           | 20.76           | 0.3501   | 1                   | em+ab              | 11.11   |
| A2192 | IJ162551.17+425622.6 | 19.23           | 21.34           | 0.3482   | -1                  | ab                 | –       |
| A2192 | IJ162551.18+425050.7 | 19.14           | 20.77           | 0.2262   | 1                   | em+ab              | 7.81    |
| A2192 | IJ162551.48+424145.3 | 18.09           | 19.55           | 0.1598   | -1                  | ab                 | –       |
| A2192 | IJ162553.24+423756.3 | 19.14           | 21.18           | 0.1855   | 1                   | ab                 | –       |
| A2192 | IJ162553.38+424822.1 | 18.05           | 20.09           | 0.1854   | -2                  | nan                | –       |
| A2192 | IJ162554.03+424039.3 | 17.89           | 20.11           | 0.1873   | 1                   | ab/em              | –       |
| A2192 | IJ162554.27+424247.3 | 18.55           | 19.73           | 0.2294   | -1                  | em                 | 17.46   |
| A2192 | IJ162554.64+425635.7 | 18.59           | 20.69           | 0.1703   | 1                   | ab                 | –       |
| A2192 | IJ162554.83+425346.6 | 19.47           | 21.62           | 0.1161   | -1                  | ab                 | –       |
| A2192 | IJ162554.92+424900.3 | 18.33           | 20.46           | 0.1884   | 1                   | ab                 | –       |
| A2192 | IJ162555.27+425747.7 | 17.53           | 19.26           | 0.1335   | 1                   | em                 | 27.9    |
| A2192 | IJ162555.60+424243.1 | 18.33           | 19.61           | 0.172    | 1                   | em                 | 12.335  |
| A2192 | IJ162556.69+421856.8 | 19.22           | 20.97           | 0.1275   | -2                  | nan                | –       |
| A2192 | IJ162557.02+422416.5 | 19.78           | 21.09           | 0.19     | -2                  | nan                | –       |
| A2192 | IJ162558.06+425319.9 | 17.57           | 19.11           | 0.1687   | 1                   | ab                 | –       |
| A2192 | IJ162558.48+425236.2 | 18.22           | 20.35           | 0.2671   | -1                  | ab                 | –       |
| A2192 | IJ162558.84+424743.6 | 19.39           | 20.63           | 0.1828   | 1                   | em                 | 28.92   |
| A2192 | IJ162559.93+424605.9 | 17.78           | 19.71           | 0.1847   | 1                   | ab                 | –       |
| A2192 | IJ162600.52+424253.9 | 19.06           | 20.28           | 0.1864   | 1                   | em                 | 13.85   |
| A2192 | IJ162600.64+421842.6 | 17.34           | 19.20           | 0.1909   | 1                   | ab/em              | 11.32   |
| A2192 | IJ162601.54+424616.6 | 19.36           | 21.45           | 0.1976   | -1                  | nan                | –       |
| A2192 | IJ162602.27+423317.6 | 19.26           | 20.90           | 0.2763   | 1                   | em+ab              | 8.8     |
| A2192 | IJ162602.29+422109.8 | 19.40           | 21.16           | 0.1901   | 1                   | em+am              | 35.72   |
| A2192 | IJ162603.49+421931.1 | 18.17           | 20.33           | 0.1892   | 1                   | ab                 | –       |
| A2192 | IJ162603.79+422905.8 | 18.53           | 19.76           | 0.1363   | 1                   | em                 | 20.6    |
| A2192 | IJ162603.82+422431.7 | 18.93           | 20.54           | 0.3261   | 1                   | em                 | 10.9    |
| A2192 | IJ162604.10+425120.7 | 19.24           | 20.87           | 0.2326   | 1                   | em+ab              | 13.7    |
| A2192 | IJ162604.72+421555.8 | 19.34           | 20.50           | 0.1328   | 1                   | em                 | 68.47   |
| A2192 | IJ162607.33+422212.4 | 18.27           | 20.43           | 0.1902   | 1                   | ab                 | –       |
| A2192 | IJ162607.63+423556.6 | 17.40           | 19.43           | 0.2252   | 1                   | em+ab              | 10.76   |
| A2192 | IJ162607.85+421854.1 | 18.79           | 20.45           | 0.1762   | -2                  | nan                | –       |
| A2192 | IJ162607.89+424128.8 | 18.09           | 19.49           | 0.1901   | 1                   | em                 | 21.91   |
| A2192 | IJ162609.63+425920.9 | 17.42           | 19.43           | 0.2349   | 1                   | em                 | 42.42   |
| A2192 | IJ162609.92+430102.1 | 18.69           | 20.87           | 0.1084   | -2                  | nan                | –       |
| A2192 | IJ162609.94+430240.5 | 19.27           | 21.27           | 0.3539   | 1                   | ab/em              | 6.47    |
| A2192 | IJ162610.26+425912.2 | 18.26           | 20.23           | 0.156    | 1                   | ab                 | –       |
| A2192 | IJ162610.25+422439.6 | 19.51           | 21.42           | 0.4527   | 1                   | em+ab              | 13.11   |
| A2192 | IJ162610.34+425416.3 | 18.87           | 21.00           | 0.1852   | 1                   | ab                 | –       |
| A2192 | IJ162610.36+422947.0 | 19.16           | 20.72           | 0.3861   | 1                   | em                 | 5.19    |
| A2192 | IJ162610.78+424916.5 | 18.35           | 20.62           | 0.2285   | 1                   | ab                 | –       |
| A2192 | IJ162612.07+425250.2 | 19.41           | 20.39           | 0.1463   | 1                   | em                 | 49.24   |
| A2192 | IJ162612.10+425149.0 | 19.32           | 20.58           | 0.1877   | 1                   | em/ab              | 33.81   |
| A2192 | IJ162614.36+424956.7 | 18.76           | 20.38           | 0.3011   | 1                   | em                 | 35.67   |
| A2192 | IJ162617.24+424025.1 | 17.61           | 18.99           | 0.1384   | -2                  | ab                 | –       |
| A2192 | IJ162618.16+423809.5 | 19.24           | 20.79           | 0.1907   | 1                   | ab/em              | 18.6    |
| A2192 | IJ162618.41+421805.8 | 18.95           | 21.00           | 0.1035   | 1                   | ab                 | –       |
| A2192 | IJ162621.85+424657.6 | 17.70           | 19.70           | 0.182    | 1                   | em+ab              | 11.6    |
| A2192 | IJ162623.43+425301.9 | 17.87           | 20.10           | 0.1867   | 1                   | ab                 | –       |
| A2192 | IJ162623.76+425321.3 | 16.45           | 18.60           | 0.1865   | -1                  | ab                 | –       |
| A2192 | IJ162623.85+424329.9 | 18.76           | 20.84           | 0.1862   | 1                   | ab/em              | 16.89   |
| A2192 | IJ162624.20+422005.7 | 19.47           | 21.32           | 0.1256   | 1                   | ab                 | –       |
| A2192 | IJ162624.56+424659.3 | 18.59           | 20.70           | 0.1906   | 1                   | ab                 | –       |

*table continues in next page...*

| Field | ID                   | <i>R</i><br>mag | <i>B</i><br>mag | redshift | redshift<br>quality | type of<br>spectra | EW[OII] |
|-------|----------------------|-----------------|-----------------|----------|---------------------|--------------------|---------|
| A2192 | IJ162624.63+425320.5 | 19.06           | 21.24           | 0.1835   | 1                   | ab                 | –       |
| A2192 | IJ162625.01+423908.0 | 19.09           | 21.20           | 0.1875   | 1                   | ab                 | –       |
| A2192 | IJ162625.42+425621.7 | 17.90           | 19.82           | 0.1847   | -1                  | nan                | –       |
| A2192 | IJ162628.24+424014.6 | 17.18           | 19.39           | 0.1872   | 1                   | ab                 | –       |
| A2192 | IJ162628.94+423848.4 | 18.82           | 21.01           | 0.1845   | 1                   | ab                 | –       |
| A2192 | IJ162629.89+423532.3 | 18.48           | 20.52           | 0.1891   | 1                   | ab                 | –       |
| A2192 | IJ162630.53+424053.1 | 19.19           | 21.26           | 0.1906   | -1                  | ab                 | –       |
| A2192 | IJ162631.73+424316.1 | 17.67           | 18.94           | 0.1914   | 1                   | em                 | 17.205  |
| A2192 | IJ162631.88+425744.8 | 18.37           | 19.84           | 0.2018   | 1                   | em                 | 26.65   |
| A2192 | IJ162632.17+425839.1 | 17.02           | 19.10           | 0.1707   | 1                   | ab                 | –       |
| A2192 | IJ162632.95+424102.7 | 18.49           | 20.62           | 0.1886   | 1                   | ab                 | –       |
| A2192 | IJ162633.05+425249.8 | 19.48           | 21.62           | 0.1239   | -1                  | ab                 | –       |
| A2192 | IJ162633.38+424045.4 | 18.94           | 21.06           | 0.1869   | 1                   | ab                 | –       |
| A2192 | IJ162634.28+424821.6 | 18.84           | 21.02           | 0.1858   | -2                  | nan                | –       |
| A2192 | IJ162634.32+424006.0 | 17.10           | 19.35           | 0.1841   | 1                   | ab                 | –       |
| A2192 | IJ162636.13+424917.7 | 18.55           | 20.76           | 0.1849   | 1                   | ab                 | –       |
| A2192 | IJ162636.68+424739.1 | 17.64           | 19.09           | 0.1074   | 1                   | em                 | 20.72   |
| A2192 | IJ162636.89+424819.8 | 18.14           | 20.32           | 0.1875   | 1                   | ab                 | –       |
| A2192 | IJ162637.37+424135.6 | 18.39           | 20.54           | 0.1909   | 1                   | ab                 | –       |
| A2192 | IJ162637.85+424201.8 | 19.15           | 21.37           | 0.2255   | 1                   | em+ab              | 14.87   |
| A2192 | IJ162637.93+424429.5 | 17.46           | 19.47           | 0.1848   | 1                   | ab                 | 0.0     |
| A2192 | IJ162638.37+425045.0 | 18.03           | 20.19           | 0.056    | 1                   | ab                 | –       |
| A2192 | IJ162638.85+422143.1 | 18.78           | 20.83           | 0.1966   | 1                   | ab                 | –       |
| A2192 | IJ162639.75+423835.2 | 19.06           | 21.28           | 0.1866   | 1                   | ab                 | –       |
| A2192 | IJ162640.29+423922.6 | 19.03           | 21.26           | 0.1849   | -1                  | ab/em              | 11.9    |
| A2192 | IJ162640.40+424538.1 | 18.67           | 20.19           | 0.2685   | -1                  | em                 | 12.2    |
| A2192 | IJ162642.56+424012.2 | 16.14           | 18.37           | 0.187    | 1                   | ab                 | –       |
| A2192 | IJ162644.40+423918.8 | 19.97           | 21.23           | 0.1906   | 1                   | em                 | 40.12   |
| A2192 | IJ162644.79+423654.6 | 18.21           | 20.00           | 0.1875   | 1                   | ab                 | 0.0     |
| A2192 | IJ162645.46+424100.6 | 18.28           | 20.37           | 0.182    | 1                   | ab                 | –       |
| A2192 | IJ162647.61+421845.5 | 18.39           | 20.50           | 0.148    | -1                  | ab                 | –       |
| A2192 | IJ162647.80+423206.3 | 18.77           | 20.31           | 0.2202   | 1                   | ab/em              | 3.62    |
| A2192 | IJ162648.36+422813.0 | 17.90           | 19.51           | 0.1253   | 1                   | em+ab              | 27.67   |
| A2192 | IJ162648.81+421839.1 | 17.68           | 19.79           | 0.16     | 1                   | ab                 | –       |
| A2192 | IJ162648.97+423738.4 | 18.64           | 20.87           | 0.1843   | 1                   | nan                | –       |
| A2192 | IJ162648.97+423630.0 | 18.88           | 21.01           | 0.1914   | 1                   | ab                 | –       |
| A2192 | IJ162649.68+424712.7 | 17.98           | 20.14           | 0.185    | -2                  | nan                | –       |
| A2192 | IJ162650.58+424320.2 | 18.98           | 21.10           | 0.1839   | 1                   | ab/em              | 7.01    |
| A2192 | IJ162651.28+422710.2 | 20.31           | 21.44           | 0.1877   | 1                   | em                 | 47.1    |
| A2192 | IJ162651.34+423437.3 | 17.85           | 19.63           | 0.1857   | 1                   | nan                | 0.0     |
| A2192 | IJ162651.52+423843.4 | 18.53           | 20.67           | 0.1865   | -1                  | ab                 | –       |
| A2192 | IJ162651.88+423950.5 | 19.41           | 21.37           | 0.1821   | 1                   | ab                 | –       |
| A2192 | IJ162652.28+423304.8 | 19.22           | 20.68           | 0.1859   | 1                   | em                 | 20.71   |
| A2192 | IJ162652.46+422703.5 | 18.75           | 19.87           | 0.1873   | 1                   | em                 | 31.09   |
| A2192 | IJ162652.57+422837.1 | 19.56           | 20.84           | 0.2213   | 1                   | em                 | 30.05   |
| A2192 | IJ162653.22+424834.9 | 18.10           | 20.17           | 0.1855   | 1                   | ab                 | –       |
| A2192 | IJ162654.47+424152.8 | 16.68           | 18.49           | 0.189    | 1                   | ab                 | 0.0     |
| A2192 | IJ162654.87+424143.6 | 18.65           | 20.07           | 0.2197   | -2                  | nan                | –       |
| A2192 | IJ162655.10+423828.5 | 18.26           | 20.35           | 0.1835   | 1                   | ab/em              | 6.27    |
| A2192 | IJ162655.54+423721.6 | 18.86           | 20.47           | 0.325    | 1                   | em                 | 12.97   |
| A2192 | IJ162657.09+424020.4 | 17.29           | 18.76           | 0.1824   | 1                   | em                 | 9.24    |
| A2192 | IJ162657.33+430333.7 | 18.05           | 19.11           | 0.2669   | -2                  | nan                | –       |
| A2192 | IJ162658.84+421557.1 | 19.37           | 21.25           | 0.1783   | -1                  | ab                 | –       |
| A2192 | IJ162703.68+424208.9 | 17.84           | 19.30           | 0.2979   | -2                  | nan                | –       |
| A2192 | IJ162704.85+421840.1 | 17.27           | 18.63           | 0.1613   | 1                   | em+ab              | 8.78    |
| A2192 | IJ162706.03+421718.3 | 17.88           | 19.87           | 0.1615   | -1                  | ab                 | –       |
| A2192 | IJ162706.94+423459.3 | 17.90           | 19.95           | 0.1865   | 1                   | ab                 | –       |
| A2192 | IJ162707.49+423936.6 | 18.87           | 19.90           | 0.1631   | 1                   | em+ab              | 14.09   |

*table continues in next page...*

| Field | ID                   | <i>R</i><br>mag | <i>B</i><br>mag | redshift | redshift<br>quality | type of<br>spectra | EW[OII] |
|-------|----------------------|-----------------|-----------------|----------|---------------------|--------------------|---------|
| A2192 | IJ162709.57+422824.5 | 18.61           | 20.68           | 0.1873   | 1                   | ab                 | –       |
| A2192 | IJ162709.63+421600.7 | 17.86           | 20.05           | 0.1895   | 1                   | ab                 | –       |
| A2192 | IJ162710.78+422754.1 | 18.14           | 19.66           | 0.1712   | -1                  | em                 | 9.76    |
| A2192 | IJ162712.05+425415.5 | 17.83           | 19.25           | 0.0898   | -2                  | nan                | –       |
| A2192 | IJ162712.25+422800.1 | 19.09           | 20.64           | 0.1332   | 1                   | ab                 | –       |
| A2192 | IJ162712.33+425206.4 | 17.91           | 20.11           | 0.2255   | 1                   | ab                 | –       |
| A2192 | IJ162712.55+424318.7 | 19.25           | 21.39           | 0.2889   | -1                  | ab                 | –       |
| A2192 | IJ162713.54+421613.1 | 19.21           | 20.70           | 0.3059   | -1                  | nan                | –       |
| A2192 | IJ162713.84+423611.2 | 18.75           | 20.10           | 0.2214   | 1                   | em+ab              | 15.34   |
| A2192 | IJ162714.06+424145.2 | 17.80           | 20.02           | 0.2328   | 1                   | ab                 | –       |
| A2192 | IJ162714.16+423612.8 | 18.03           | 20.02           | 0.2206   | 1                   | ab                 | –       |
| A2192 | IJ162714.24+421840.8 | 19.49           | 21.03           | 0.1583   | 1                   | ab                 | –       |
| A2192 | IJ162716.19+423303.9 | 18.06           | 20.19           | 0.1863   | 1                   | ab                 | –       |
| A2192 | IJ162716.24+424801.2 | 18.24           | 20.46           | 0.2227   | 1                   | ab                 | –       |
| A2192 | IJ162717.29+421720.5 | 17.58           | 19.21           | 0.1555   | 1                   | ab/em              | 7.08    |
| A2192 | IJ162717.72+430309.2 | 18.24           | 19.72           | 0.2275   | 1                   | em                 | 32.26   |
| A2192 | IJ162719.24+425051.2 | 17.98           | 19.87           | 0.1569   | 1                   | ab                 | –       |
| A2192 | IJ162719.72+425146.7 | 18.08           | 20.27           | 0.225    | 1                   | ab                 | –       |
| A2192 | IJ162721.05+425506.7 | 18.56           | 20.62           | 0.2232   | -1                  | ab                 | –       |
| A2192 | IJ162722.70+424125.7 | 17.79           | 19.28           | 0.2323   | 1                   | em                 | 49.69   |
| A2192 | IJ162723.30+423318.8 | 18.56           | 20.40           | 0.1864   | 1                   | em+ab              | 8.71    |
| A2192 | IJ162723.76+423838.5 | 19.04           | 20.96           | 0.2698   | 1                   | em/ab              | 26.44   |
| A2192 | IJ162723.86+422236.4 | 17.94           | 19.97           | 0.1852   | 1                   | ab                 | –       |
| A2192 | IJ162724.99+424806.1 | 19.48           | 21.22           | 0.2471   | 1                   | em                 | 33.18   |
| A2192 | IJ162725.09+430142.1 | 18.82           | 20.49           | 0.3287   | 1                   | em                 | 14.49   |
| A2192 | IJ162725.73+430318.7 | 19.47           | 20.60           | 0.0917   | 1                   | em                 | 108.6   |
| A2192 | IJ162726.74+423229.6 | 18.98           | 20.55           | 0.158    | 1                   | ab                 | –       |
| A2192 | IJ162727.02+423232.0 | 17.75           | 19.73           | 0.159    | 1                   | ab                 | –       |
| A2192 | IJ162727.58+423750.3 | 18.20           | 19.63           | 0.2319   | -2                  | nan                | –       |
| A2192 | IJ162729.89+425747.2 | 18.45           | 19.96           | 0.17     | 1                   | em                 | 32.7    |
| A2192 | IJ162730.82+422516.3 | 18.57           | 20.73           | 0.1894   | 1                   | nan                | –       |
| A2192 | IJ162732.09+424830.3 | 18.44           | 20.36           | 0.2249   | 1                   | em+ab              | 12.54   |
| A2192 | IJ162732.44+430020.1 | 19.26           | 20.75           | 0.276    | -1                  | nan                | –       |
| A2192 | IJ162735.51+425640.2 | 18.90           | 20.91           | 0.3042   | -2                  | nan                | –       |
| A2192 | IJ162736.58+425913.2 | 18.74           | 19.81           | 0.0606   | -1                  | na                 | –       |
| A2192 | IJ162740.09+425107.3 | 19.50           | 21.21           | 0.2171   | -2                  | nan                | –       |
| A2192 | IJ162740.15+423008.8 | 18.95           | 20.04           | 0.1331   | 1                   | em                 | 26.52   |
| A2192 | IJ162740.45+422252.3 | 18.31           | 20.35           | 0.1894   | 1                   | ab                 | –       |
| A2192 | IJ162741.20+422248.2 | 19.15           | 20.71           | 0.2009   | -1                  | ab                 | –       |
| A2192 | IJ162741.79+424832.1 | 19.03           | 20.40           | 0.157    | 1                   | em                 | 29.14   |
| A2192 | IJ162742.31+423207.7 | 18.74           | 20.09           | 0.2265   | 1                   | em+ab              | 12.44   |
| A2192 | IJ162744.27+421922.7 | 18.39           | 19.49           | 0.1677   | 1                   | nan                | –       |
| A2192 | IJ162744.94+422716.1 | 19.43           | 20.97           | 0.2497   | 1                   | em                 | 17.4    |
| A2192 | IJ162745.00+425434.5 | 17.95           | 19.40           | 0.1093   | -2                  | nan                | –       |
| A2192 | IJ162745.36+423204.4 | 18.97           | 20.56           | 0.2693   | 1                   | em+ab              | 8.0     |
| A2192 | IJ162745.49+425450.8 | 16.46           | 18.00           | 0.1022   | -2                  | nan                | –       |
| A2192 | IJ162749.86+423825.9 | 17.35           | 18.65           | 0.1722   | 1                   | em                 | 23.54   |
| A2192 | IJ162750.24+430106.3 | 19.13           | 20.23           | 0.1892   | 1                   | em                 | 62.71   |
| A2192 | IJ162751.97+425310.3 | 17.86           | 19.93           | 0.1567   | -1                  | ab                 | –       |
| A2192 | IJ162752.56+424108.5 | 18.78           | 20.20           | 0.1256   | -2                  | nan                | –       |
| A2192 | IJ162753.06+422239.3 | 18.86           | 20.92           | 0.2327   | 1                   | ab                 | –       |
| A2192 | IJ162756.84+424726.7 | 18.08           | 19.81           | 0.1386   | -1                  | nan                | –       |
| A2192 | IJ162758.41+424740.8 | 18.53           | 20.47           | 0.1339   | -2                  | nan                | –       |
| A2192 | IJ162759.62+424253.8 | 19.43           | 21.35           | 0.343    | 1                   | em+ab              | 8.85    |
| A2192 | IJ162800.29+424103.4 | 18.10           | 19.47           | 0.1367   | 1                   | ab                 | –       |
| A2192 | IJ162800.93+425328.5 | 19.13           | 21.19           | 0.3452   | -2                  | nan                | –       |
| A2192 | IJ162802.89+423705.4 | 19.07           | 20.44           | 0.2323   | 1                   | em                 | 28.67   |
| A2192 | IJ162803.56+425027.1 | 18.08           | 19.72           | 0.0498   | 1                   | ab                 | –       |

*table continues in next page...*

| Field | ID                   | <i>R</i><br>mag | <i>B</i><br>mag | redshift | redshift<br>quality | type of<br>spectra | EW[OII] |
|-------|----------------------|-----------------|-----------------|----------|---------------------|--------------------|---------|
| A2192 | IJ162804.98+423658.9 | 17.98           | 20.15           | 0.2319   | 1                   | ab                 | –       |
| A2192 | IJ162806.05+425347.4 | 18.25           | 20.41           | 0.2586   | -2                  | nan                | –       |
| A2192 | IJ162808.18+424020.2 | 18.25           | 20.50           | 0.3514   | 1                   | ab                 | –       |
| A2192 | IJ162809.26+422446.4 | 18.93           | 20.07           | 0.1478   | -1                  | ab                 | –       |
| A2192 | IJ162809.35+425457.4 | 17.76           | 19.24           | 0.2544   | 1                   | em                 | 12.45   |
| A2192 | IJ162809.48+423040.1 | 19.21           | 20.48           | 0.2129   | 1                   | em                 | 25.87   |
| A2192 | IJ162809.57+422256.4 | 19.17           | 21.08           | 0.1555   | -2                  | nan                | –       |
| A2192 | IJ162811.22+425745.9 | 17.61           | 18.84           | 0.1343   | 1                   | nan                | –       |
| A2192 | IJ162812.10+423725.4 | 19.41           | 21.09           | 0.2922   | -1                  | nan                | –       |
| A2192 | IJ162813.09+424933.3 | 19.19           | 20.77           | 0.225    | 1                   | em+ab              | 26.62   |
| A2192 | IJ162813.23+424311.6 | 19.29           | 20.67           | 0.2309   | 1                   | em                 | 30.96   |
| A2192 | IJ162815.54+424801.9 | 18.77           | 20.81           | 0.2123   | -1                  | ab                 | –       |
| A2192 | IJ162815.65+425248.7 | 19.12           | 20.90           | 0.2767   | 1                   | ab                 | –       |
| A2192 | IJ162815.75+425347.4 | 19.14           | 20.88           | 0.2778   | -1                  | em                 | 31.34   |
| A2192 | IJ162819.80+424203.4 | 18.33           | 19.91           | 0.275    | 1                   | em                 | 16.195  |
| A2192 | IJ162820.58+425133.4 | 18.44           | 20.42           | 0.155    | 1                   | ab                 | –       |
| A2192 | IJ162821.23+422744.7 | 18.89           | 20.30           | 0.2698   | 1                   | em                 | 33.62   |
| A2192 | IJ162823.32+425225.8 | 18.81           | 20.72           | 0.23     | -2                  | nan                | –       |
| A2192 | IJ162824.75+424346.6 | 18.99           | 20.15           | 0.1413   | -1                  | ab                 | –       |
| A2192 | IJ162830.28+425120.5 | 18.41           | 20.41           | 0.2282   | -2                  | nan                | –       |
| A2192 | IJ162836.67+423517.4 | 18.58           | 20.78           | 0.2308   | 1                   | ab                 | –       |
| A2192 | IJ162839.15+423638.4 | 19.19           | 21.35           | 0.2167   | -1                  | ab                 | –       |
| A2192 | IJ162839.52+423854.7 | 17.58           | 19.07           | 0.1159   | 1                   | ab/em              | 5.59    |
| A2192 | IJ162839.56+424902.3 | 19.40           | 21.20           | 0.3691   | 1                   | em/ab              | 29.26   |
| A2192 | IJ162843.31+424908.4 | 18.73           | 20.51           | 0.235    | 1                   | ab                 | –       |
| A2192 | IJ162843.41+424030.3 | 19.08           | 21.35           | 0.1502   | -1                  | ab                 | –       |
| A2192 | IJ162844.98+423541.9 | 17.91           | 19.48           | 0.2269   | 1                   | em                 | 16.81   |
| A2192 | IJ162845.23+423650.3 | 19.44           | 21.04           | 0.3418   | 1                   | em                 | 34.33   |
| A2192 | IJ162846.78+423332.2 | 19.16           | 20.98           | 0.3262   | 1                   | em/ab              | 12.63   |
| A2192 | IJ162531.48+422850.0 | 18.25           | 20.37           | 0.1104   | -1                  | nan                | –       |
| A2192 | IJ162708.18+422217.0 | 17.22           | 18.38           | 0.1359   | -1                  | ab                 | –       |
| A2192 | IJ162700.55+424047.0 | 18.15           | 19.87           | 0.2311   | 1                   | em                 | 36.83   |
| A2192 | IJ162531.52+423913.2 | 19.37           | 20.82           | 0.2008   | -1                  | ab                 | –       |
| A2192 | IJ162719.62+422033.7 | 18.99           | 21.06           | 0.2302   | -1                  | ab                 | –       |
| A2192 | IJ162746.54+425603.6 | 18.92           | 20.53           | 0.1403   | -1                  | ab                 | –       |
| A2192 | IJ162720.80+422112.5 | 19.20           | 20.75           | 0.1345   | -1                  | nan                | –       |
| A2192 | IJ162700.98+424111.0 | 19.26           | 20.91           | 0.533    | -2                  | ab                 | –       |
| A2192 | IJ162653.33+424206.9 | 18.87           | 20.58           | 0.3304   | -2                  | nan                | –       |
| A2192 | IJ162710.28+425407.8 | 19.18           | 20.39           | 0.1657   | -2                  | em/ab              | 15.9    |
| A2192 | IJ162639.95+424148.1 | 18.81           | 20.26           | 0.2249   | 1                   | em                 | 12.91   |
